# Supplementary material for: Aspects of Quantum Cosmology
Source: arXiv:2101.12659 source file (2021-01-29)
Supplement: Supplementary file 1 [file appendix.tex]

\setcounter{equation}{0}  % reset counter

\setcounter{figure}{0}  % reset counter

\chapter*{Appendix}\label{ch:appendix}\addcontentsline{toc}{chapter}{Appendix}

\chaptermark{Appendix}
\sectionmark{Appendix}
\vspace{-1.3cm}

In this ~\nameref{ch:appendix} we present the calculations other Bianchi models for Chap. \ref{ch4:1}.

%\section*{3. Calculation of elastic free energy}\label{sec:app_felastic}
